# Supplementary material for: A Two-Ball Ellsberg Paradox: An Experiment
Source: arXiv:2206.04605 source file (2022-11-21)
Supplement: Supplementary file 1 [file Appendices_AnalysisReplicationFile.tex]

\documentclass[10pt]{article}

\usepackage{amssymb,amsmath,amsfonts,eurosym,geometry,ulem,graphicx,caption,color,setspace,sectsty,comment,footmisc,caption,natbib,pdflscape,subfigure,array,hyperref,theorem, kpfonts, appendix, xcolor, tabularx, cellspace, setspace, booktabs, makecell, fancyhdr, enumitem, pdflscape, adjustbox, rotating}

\normalem

\onehalfspacing

\theorembodyfont{\rm}

\newcolumntype{L}[1]{>{\raggedright\let\newline\\arraybackslash\hspace{0pt}}m{#1}}
\newcolumntype{C}[1]{>{\centering\let\newline\\arraybackslash\hspace{0pt}}m{#1}}
\newcolumntype{R}[1]{>{\raggedleft\let\newline\\arraybackslash\hspace{0pt}}m{#1}}

\geometry{left=1.2in,right=1.2in,top=1.0in,bottom=1.0in}

%My Commands--------------------------------------------------------------------------------
\usepackage [english]{babel}
\usepackage [autostyle, english = american]{csquotes}
\MakeOuterQuote{"}

\usepackage[utf8]{inputenc}
\usepackage{natbib}
\bibliographystyle{te}

\usepackage{bbm}
\usepackage{comment}
\usepackage{enumerate}
\usepackage{nameref}

\definecolor{softblue}{HTML}{1C46C0}
\hypersetup{%
  colorlinks = true,
  linkcolor= softblue, 
  citecolor = softblue
}

\setlength\cellspacetoplimit{10pt}
\setlength\cellspacebottomlimit{10pt}

\pagestyle{fancy}
\lhead{\sc a two-stage ellsberg paradox}
\rhead{\sc analysis replication file}

%Title Page-----------------------------------------------------------------------------------
\begin{document}
\title{\sc \textbf{appendices} \\
replication file}
\date{\today}
\maketitle
\tableofcontents
\listoftables
\newpage

\newpage
\section{Analysis with Representative Sample, n = 400}
We make the following analysis as follows. First, we drop all observations which have at least one $P^j = 0$. Then, we do all the analysis with $I^A = 1$ and one with  $I^A = 0$
\subsection{Descriptive Statistics}
\subsubsection{Summary Statistics}
\begin{itemize}
    \item \textcolor{red}{Report the CDF of $T^j_i$. Is KK just due to random chance?}
    \item Report the average of all the $T^j_i$ variables (i.e. across all participants, both elicitations, all treatments), as well as a 95\% confidence interval for this average.  (This being positive means on average, \textit{all} people pay more for $KK$ than $UU$.)
    \item Do the same for the averages of all the $E_i^j$'s, $H_i^j$'s and $L_i^j$'s.  Note that when computing things about $H$ and $L$, use only the data from that one treatment.  (These averages equal the \textit{proportions} of subjects who fall for the various traps.)
\end{itemize}

\subsubsection{Measurement Error}
    \begin{itemize}
    \item Report the correlation ($r$) between $T^1$ and $T^2$.  (1 minus this correlation gives "the fraction of variation in $T$ that's due to noise." (See Page 28 of "Testing the Waters.") So having high $r$ is good.)
    \item Also report the standard error of this coefficient.  In case Stata doesn't have a formula for this, it's
    \[ \sqrt{\frac{1-r^2}{n-2}}. \]
    \item Do the same for $E$, $H$, and $L$.
    \bigskip
\end{itemize}

\textcolor{red}{\subsection{Main Regressions for $T$ as Dependent Variable}}

\begin{itemize}
    \item For all regressions for $T$ as dependent variable, we will have two main tables. One in a simple regression type, one in a combined regression type. Before describing the regressions we intend to run, we briefly discuss this distinction. For single regressions, put the coefficient from the regression where you use only that one variable (i.e. the regression is  $T = \beta_0 + \beta_1 X + \epsilon$ where in each row X will equal the one variable on the left column of that row in the table above).  For combined regressions, include all of them in one regression.
    \item Run all regressions using the ORIV approach when we have two elicitations. 
    \item Report the correlation from the ORIV regressions.
\end{itemize}

\subsubsection{Use Main Failures: E, H, L}
$T = \beta_0 + \beta_1 E + \beta_2 H + \beta_1 L + \epsilon$
combining the two elicitations with 2SLS. 

\subsubsection{Add Main Controls}
 run the same as in 2.3.1 but now add ''attention checks'', $I^A$ ($A^j=1$), ``cognitive test'', $I^R$ ($R^2=1$ and $R^3=0$) and  ``risk aversion'', $K$ ($Balc1a$ and $Final1a$).

\subsubsection{Add UK and KU}
run the same as in 2.3.2 but now add $UK$ ($Balu1c$ and $Matu1c$) and $KU$ ($Balu1d$ and $Matu1d$).

\subsubsection{Add Independent Urns}
run the same as in 2.3.3 but now add $II$ ($Balu4$). 

\subsubsection{Add Demographics}
run the same as in 2.3.4 but now add ``Demographics'' ($Age$ and $Gender$).

\subsection{Other Regressions for $T$ as Dependent Variable}

\subsubsection{Learning Effects}
$T = \beta_0 + \beta_1 I^B + \epsilon$. \ \ \ \ \ \ ($\beta_1$ being $<0$ and significant means that being in the "learning" treatment has a causal effect of reducing how often they fall for the 2Ellsberg trap.).

\textcolor{red}{\subsubsection{Amount of Ambiguity}}
First, present histograms of $\frac{KK^1 + KK^2}{2}$, $\frac{UU^1 + UU^2}{2}$, $KKK$, $UUU$, and $KUU$.  Use the combined data from \textit{all four} treatments for the first two of these, and only the data from treatment D for the last three (as we only have data on these in treatment D).

Report 95\% confidence intervals for each of the following things.  In each case, report three versions of the confidence interval: (1) among \textit{all} people in treatment D, (2) among those people in treatment D who had $I^T = 1$ (i.e. "fell for the 2-Ellsberg trap"), and (3) among those people in treatment D who had $I^T = 0$.
\begin{itemize}
    \item $\overline{F^{1-3}}-\overline{F^{0-2}}$ \ \ \ (That is, for each person $i$, let $D_i = F^{1-3}_i - F^{0-2}_i$ be that person's difference of these variables.  Then report a 95\% confidence interval for $\overline{D}$, the \textit{average} of these differences across people in treatment D.)
    \item $\overline{F^{0-3}}-\overline{F^{0-2}}$
\end{itemize}
In each case, report the $p$-value for the hypothesis test of "Null hypothesis: $\overline{D} = 0$."

\bigskip
\bigskip
Next, move to the data on "bounded U" stuff in treatment C.  Report histograms of $BB^{40-60}$, $BB^{60-100}$ and $BB^{95-100}$.  (This will only involve data from treatment C.)

Then, report 95\% confidence intervals for each of the following things.  In each case, report three versions of the confidence interval: (1) among \textit{all} people in treatment C, (2) among those people in treatment C who had $I^T = 1$ (i.e. "fell for the 2-Ellsberg trap"), and (3) among those people in treatment C who had $I^T = 0$.
\begin{itemize}
    \item $\overline{BB^{40-60}}-\overline{UU}$ \ \ \ (That is, for each person $i$, let $D_i = BB^{40-60}_i - UU_i$ be that person's difference of these variables.  Then report a 95\% confidence interval for $\overline{D}$, the \textit{average} of these differences across people in treatment C.)
    \item $\overline{BB^{60-100}}-\overline{UU}$
    \item $\overline{BB^{60-100}}-\overline{BB^{40-60}}$
    \item $\overline{BB^{95-100}}-\overline{BB^{60-100}}$
\end{itemize}
In each case, report the $p$-value for the hypothesis test of "Null hypothesis: $\overline{D} = 0$."

\subsection{Other Regressions}
\begin{itemize}
    \item Run ORIV regressions with ...
\end{itemize}

\newpage
%%%%%%%%%%%%%%%%
\begin{appendices}
\section{Empirical Strategy}
\subsection{Choosing KK or UU}
\paragraph{\textbf{\textsc{aim}}}Do subjects sometimes choose to avoid an ambiguous act by choosing an unambiguous lottery that is worse than any lottery the ambiguous act could produce?

\paragraph{\textbf{\textsc{how}}}

\paragraph{\sc definitions}

Let $K_i$ be person $i$'s CE for KK, and $U_i$ be her CE for UU (both estimated using Yariv technique).  Then let
\[ D_i = K_i - U_i \]
be the difference between these CEs.  Thus, $D_i > 0$ means $i$ prefers KK to UU, and larger values of $D_i$ mean stronger preference for KK over UU.

Let $F_i = 1$ if $D_i > 0$, i.e. if person $i$ chooses KK over UU.

\paragraph{how}
First thing: Test $H_0 : D_i = 0$ vs. $H_A : D_i > 0$.  I suspect we will fail to reject $H_0$, simply because only CERTAIN people will fall for the trap.

\paragraph{how}
Similarly: Present proportion of people who have $F_i = 1$.  Could also do this within each treatment, and just for 1st measurement vs second measurement.

\paragraph{how}
Also: Split subjects into 2 groups: those with $D_i > 0$ and those with $D_i \leq 0$.  Then test whether $D$ is the same among the two groups, or not.

\subsection{Explaining KK}
\paragraph{\textbf{\textsc{aim}}}Can subjects' "irrational" choices in (1) be explained by whether they engage in other more classically "irrational" modes of behavior, such as failing to reduce compound lotteries or being ambiguity averse in the classic Ellsberg paradox?

\paragraph{\textbf{\textsc{how}}}

\paragraph{\sc Definitions}Define $A_i$ = $i$'s CE for K Ellsberg urn gamble, and $B_i$ = $i$'s CE for U Ellsberg gamble (i.e. a 50-50).  Then let
\[ C_i = A_i - B_i \]
be the difference.  That is, $C_i > 0$ means $i$ prefers K to U, and larger $C_i$ means stronger preference for $K$ over $U$.

\noindent We now list the regressions we want to run.

\paragraph{Level differences: 2Ellsberg vs. 1Ellsberg}
Basic regression on CEs:
\[ D_i = \beta_0 + \beta_1 C_i + \epsilon_i \]
and test whether $\beta_1 > 0$.

\paragraph{Frequency differences: 2Ellsberg vs. 1Ellsberg}
Basic regression on frequencies:
Recall $F_i = 1$ if $D_i > 0$ (i.e. if you fall for 2Ellsberg paradox).  Now, let $G_i = 1$ if $C_i > 0$ (i.e. if you fall for classic Ellsberg paradox).  We can do a logit/probit regression of $F_i$ on $G_i$.

\paragraph{Correlation}
Also, compute correlation between $F_i$ and $G_i$.

\paragraph{Level and Frequency Differences: 2Ellsberg vs. Halevy}
Next, using data from treatment 2 (compound lotteries), we can do the analogous regressions.  Let $W_i$ = CE for Halevy compound lottery, and $A_i$ = CE for simple 50-50.  Then we can let $E_i = A_i - W_i$, so $E_i > 0$ means you prefer a simple 50-50 to a compound 50-50.  Then we can do the same kinds of regressions with $E_i$ (or its indicator variable for being $>0$) in place of $C_i$ or $G_i$.  For example,
\[ D_i = \beta_0 + \beta_1 E_i + \epsilon_i. \]
Run this regression using only those people in treatment 2.

\subsection{Amount of Ambiguity}
\paragraph{\textbf{\textsc{aim}}}How do subjects' willingness to pay to avoid ambiguity change as a function of the "amount of ambiguity" in the situations they face?

\paragraph{\textbf{\textsc{how}}}

\paragraph{\sc definitions}

\paragraph{regression....}

\subsection{Learning}
\paragraph{\textbf{\textsc{aim}}}Do subjects learn to avoid making the "irrational" choice in (1) if they are exposed beforehand to similar choice problems that highlight the fact that the ambiguous act can "only be better"?
\paragraph{\textbf{\textsc{how}}}
\paragraph{\sc definitions}
Let $I_i = 1$ if $i$ is in treatment 3 ("teaching" treatment), and 0 otherwise.  

\paragraph{blabla....}
Then run the regression
\[ D_i = \beta_0 + \beta_1 I_i + \epsilon_i \]
Here, $\beta_1 < 0$ (and statistically significant) would mean that being in treatment 3 causes a significant reduction in how strongly you fall for the 2Ellsberg trap.

\paragraph{blabla....}
Similarly, we can run a logit/probit regression of $F_i$ on $I_i$.  The coefficient being $<0$ (and significant) would mean that being in treatment 3 makes you less likely to fall for the 2Ellsberg trap.

\subsection{Robustness checks / mental processes}
KU, UK, II stuff

\newpage
Other important data checks:
-Do people treat UU the same as KU / UK?  How about two independent ambiguous urns?
\end{appendices}

\end{document}
