# Supplementary material for: A Two-Ball Ellsberg Paradox: An Experiment
Source: arXiv:2206.04605 source file (2022-11-21)
Supplement: Supplementary file 2 [file OnlineAppendices.tex]

\documentclass[10pt]{article}

\usepackage{amssymb,amsmath,amsfonts,eurosym,geometry,ulem,graphicx,caption,color,setspace,sectsty,comment,footmisc,caption,natbib,pdflscape,subfigure,array,hyperref,theorem, kpfonts, xcolor, tabularx, cellspace, setspace, booktabs, makecell, fancyhdr, enumitem, pdflscape, adjustbox, rotating}

\usepackage[toc,page]{appendix}

\normalem

\onehalfspacing

\theorembodyfont{\rm}

\newcolumntype{L}[1]{>{\raggedright\let\newline\\arraybackslash\hspace{0pt}}m{#1}}
\newcolumntype{C}[1]{>{\centering\let\newline\\arraybackslash\hspace{0pt}}m{#1}}
\newcolumntype{R}[1]{>{\raggedleft\let\newline\\arraybackslash\hspace{0pt}}m{#1}}

\geometry{left=1.2in,right=1.2in,top=1.0in,bottom=1.0in}

%My Commands--------------------------------------------------------------------------------
\usepackage [english]{babel}
\usepackage [autostyle, english = american]{csquotes}
\MakeOuterQuote{"}

\usepackage[utf8]{inputenc}
\usepackage{natbib}
\bibliographystyle{te}

\usepackage{bbm}
\usepackage{comment}
\usepackage{enumerate}
\usepackage{nameref}

\definecolor{softblue}{HTML}{1C46C0}
\definecolor{softred}{HTML}{B54747}

\hypersetup{%
  colorlinks = true,
  linkcolor = softblue,
  citecolor = softred
}

\begin{document}

\begin{titlepage}
\title{\textsc{\bfseries \Large online appendix} \\[6pt]
\sc  a two-stage ellsberg paradox \\[6pt]
\large \textit{Evidence from an US Representative Sample}}
\vspace{10in}
\author{Brian Jabarian\thanks{Princeton University} \hspace{35pt} Simon Lazarus\thanks{Princeton University}}
\date{\today}
\maketitle

\begin{spacing}{1.2}
\fontsize{9pt}{12pt}\selectfont
\tableofcontents
\end{spacing}

\setcounter{page}{0}
\thispagestyle{empty}
\end{titlepage}
\pagebreak \newpage

\doublespacing

\include{Appendices_Main}
\include{Appendices_DataCollectionDetails}
\include{Appendices_Dictionnary}
\section{Prolific Pilot Test Sample}
\subsection{Summary Statistics}
\begin{sidewaystable}
\centering
\scriptsize
\caption{\sc summary statistics for pilot, n=100}
\begin{tabular}{lccccccccccc}
\addlinespace
\toprule \toprule
\addlinespace
& \multicolumn{2}{c}{$ I^A = 0 $} &       & \multicolumn{2}{c}{$ I^A = 1 $} &       & \multicolumn{2}{c}{$ I^A = 0 $ } &       & \multicolumn{2}{c}{$ I^A = 1 $ } \\
\cmidrule{2-3}\cmidrule{5-6}\cmidrule{8-9}\cmidrule{11-12}      & $  E^1$  & $  E^2$  &       & $  E^1$  & $  E^2$  &       & $ T^1$  & $ T^2$  &       & $ T^1$  & $ T^2$  \\
\midrule
Mean  &     2.00    &   18.00     &  &    5.62    &    7.88   &  &   4.00    &  -28.20     &  &    9.18    &    9.39   \\
$ 95\%$  Conf. Interval &  [-11.60 ,  15.60 ]   &   [-20.67 ,  56.67 ]    &   & [ -5.31 ,  16.56 ]   &   [ -2.76 ,  18.52 ]   &   & [-14.83 ,  22.83 ]   &   [-136.42 ,  80.02 ]    &   & [ -0.99 ,  19.34 ]   &   [ -1.50 ,  20.28 ]  \\
N     &   5    &  5  & &  85    &  85    &  &   5    &  5  & &  85    &  85  \\
&    \\
& \multicolumn{2}{c}{$  I^A = 0 $ } &       & \multicolumn{2}{c}{$  I^A = 1 $ } &       & \multicolumn{2}{c}{$ I^A = 0 $ } &       & \multicolumn{2}{c}{$ I^A = 1 $ } \\
\cmidrule{2-3}\cmidrule{5-6}\cmidrule{8-9}\cmidrule{11-12}      & $  H^1$  & $  H^2$  &       & $  H^1$  & $  H^2$  &       & $ L^1$  & $ L^2$  &       & $ L^1$  & $ L^2$  \\
\midrule
Mean  &     0.00    &   20.00     &  &   25.17    &    3.04   &  &   0.00    &    0.00     &  &   -4.39    &   11.26   \\
$ 95\%$  Conf. Interval &    [     . ,      . ]   &   [     . ,      . ]    &   & [ -6.71 ,  57.06 ]   &   [-27.42 ,  33.51 ]   &   & [     . ,      . ]   &   [     . ,      . ]    &   & [-38.88 ,  30.10 ]   &   [-19.34 ,  41.86 ]  \\
N     &   1    &  1  & &  23    &  23    &  &   1    &  1  & &  23    &  23  \\
\addlinespace
\bottomrule \bottomrule
\end{tabular}
\end{sidewaystable}
\newpage

\subsection{ORIV Correlations}
\begin{table}[ht][ht]
\centering
\footnotesize
\caption{\sc corrected oriv correlations for pilot, n=100}
\begin{tabular}{lccccccc}
\addlinespace
\toprule \toprule
\addlinespace
& \multicolumn{3}{c}{$ I^A = 0 $} &       & \multicolumn{3}{c}{$ I^A = 1 $} \\
\cmidrule{2-4}\cmidrule{6-8}Variables & $ \rho $ & $ 1-\rho $ & se $ 1-\rho $ & & $ \rho $ & $ 1-\rho $ & se $ 1-\rho $ \\
\midrule
$ E^1 $ \& $ E^2 $ &  0.088 &  0.912 &  0.575 & &  0.119 &  0.881 &  0.109 \\
$ T^1 $ \& $ T^2 $ & -0.996 &  1.996 &  0.052 & &  0.280 &  0.720 &  0.105 \\
$ H^1 $ \& $ H^2 $ &  &  &  & &  0.169 &  0.831 &  0.215 \\
$ L^1 $ \& $ L^2 $ &  &  &  & &  0.632 &  0.368 &  0.169 \\
\addlinespace
\bottomrule \bottomrule
\end{tabular}
\end{table}
\newpage

\subsection{Main Regressions: $T$ as Dependent Variable}
\begin{table}[ht]
\centering
\footnotesize
\caption{\sc Dependent Variable $T$, for pilot, n=100}
\begin{tabular}{lccccccccccccccc}
\addlinespace
\toprule \toprule
\addlinespace
\multicolumn{16}{c}{Dependent Variable: $T$} \\
\midrule
& $ I^A = 0 $ &       & $ I^A = 1 $ &       & $ I^A = 0 $ &       & $ I^A = 1 $ &       & $ I^A = 0 $ &       & $ I^A = 1 $ &       & $ I^A = 0 $ &       & $ I^A = 1 $ \\
\cmidrule{2-2}\cmidrule{4-4}\cmidrule{6-6}\cmidrule{8-8}\cmidrule{10-10}\cmidrule{12-12}\cmidrule{14-14}\cmidrule{16-16}
Ind. Variable $ j $ &     $ E $ &           & $ E $ &               & $ T $ &                    & $ T $ &                   & $ H $ &         & $ H $ &                             & $ L $ &          & $ L $ \\
\midrule
$ I^{j} $   &  & &  0.457** & &  & &  1.181*** & &  & &  1.100 & &  & &  1.865  \\
&                        & & (0.181)               & &                    & & (0.265)               & &                & & (1.247)               & &            & & (1.549)  \\
ORIV Coeff. &                & & .651               & &                    & & 1.573               & &                & & .6149               & &            & & 1.1974  \\
\midrule
$ N  $      & 0                       & & 64               & & 0                   & & 64               & & 0                   & & 23               & & 0                   & & 23  \\
\addlinespace
\bottomrule \bottomrule
\end{tabular}
\end{table}
\newpage

\subsection{Other Regressions: $E$, $H$ and $L$ as Dependent Variables}
\begin{table}[ht]
\centering
\footnotesize
\caption{\sc for pilot, n=100}
\begin{tabular}{lccccccccccccccc}
\addlinespace
\toprule \toprule
\addlinespace
& $ I^A = 0 $ &       & $ I^A = 1 $ &       & $ I^A = 0 $ &       & $ I^A = 1 $ &       & $ I^A = 0 $ &       & $ I^A = 1 $ &       & $ I^A = 0 $ &       & $ I^A = 1 $ \\
\cmidrule{2-2}\cmidrule{4-4}\cmidrule{6-6}\cmidrule{8-8}\cmidrule{10-10}\cmidrule{12-12}\cmidrule{14-14}\cmidrule{16-16}Variable & $ E $ &       & $ E $ &       & $ T $ &       & $ T $ &       & $ H $ &       & $ H $ &       & $ L $ &       & $ L $ \\
\midrule
$ I^{j} $   &    & &  1.024***   & &    & &  1.181***   & &    & &  2.576   & &    & &  1.869  \\
&        & & (0.205)   & &    & & (0.265)   & &    & & (2.846)   & &    & & (1.571)  \\
ORIV Coeff. &    & & 1.3976   & &    & & 1.573   & &    & & 2.5284   & &    & & 1.0888  \\
\midrule
$ N  $      & 0   & & 64   & & 0   & & 64   & & 0   & & 23   & & 0   & & 23  \\
\addlinespace
\bottomrule \bottomrule
\end{tabular}
\end{table}
\newpage

\subsection{Learning Effects}
\begin{table}[ht]
\centering
\footnotesize
\caption{\sc learning effects for pilot, n=100}
\begin{tabular}{lcc}
\addlinespace
\toprule \toprule
\addlinespace
&\multicolumn{1}{c}{$ T^{1} $ }  & \multicolumn{1}{c}{$ T^{2} $ }         \\
\midrule
$ I^{B} $  &      -21.343*     &        -4.024      \\
&     (10.925)    &     (12.903)         \\
\addlinespace
Const.     &      14.343**      &      8.328            \\
&     (5.523)   &     (6.523)         \\
\midrule
$ N  $     &          90         &          90         \\
\addlinespace
\bottomrule \bottomrule
\end{tabular}
\end{table}

\end{document}
